# Supplementary material for: Identifiability of AMP chain graph models
Source: arXiv:2106.09350 source file (2021-06-17)
Supplement: Supplementary file 1 [file appendix.tex]

\appendix
% NOTE: necessary when ptmx or no mathfont class option is given
\providecommand{\upGamma}{\Gamma}
\providecommand{\uppi}{\pi}
\section{Math font exposition}
How math looks in equations is important:
\begin{equation*}
  F_{\alpha,\beta}^\eta(z) = \upGamma(\tfrac{3}{2}) \prod_{\ell=1}^\infty\eta \frac{z^\ell}{\ell} + \frac{1}{2\uppi}\int_{-\infty}^z\alpha \sum_{k=1}^\infty x^{\beta k}\mathrm{d}x.
\end{equation*}
However, one should not ignore how well math mixes with text:
The frobble function \(f\) transforms zabbies \(z\) into yannies \(y\).
It is a polynomial \(f(z)=\alpha z + \beta z^2\), where \(-n<\alpha<\beta/n\leq\gamma\), with \(\gamma\) a positive real number.
